# Supplementary material for: High-order accurate schemes for Maxwell's equations with nonlinear active media and material interfaces
Source: arXiv:2108.09519 source file (2021-08-21)
Supplement: Supplementary file 1 [file secondOrderSupplemental.tex]

\section{Supplemental Equations for Second-Order}
\label{sec:2ndsupp}

{\bf Words saying that these are the bits needed to complete the 2nd order scheme.}
\begin{subequations}
\begin{align}
  \left.D_{2t}N_\ell\right|^n_{\jv} &\defeq \sum_{\hat{\ell}}\alpha_{\ell,\hat{\ell}}N^n_{\hat{\ell},\jv} + \sum_{m}\beta_{\ell,m}\Ev^n_{\jv}\cdot D_{0t} \Pv^n_{m,\jv},\label{eqn:2-accurate-Nt}\\
  \left.D_{2tt}N^{n}_\ell\right|_{\jv}^n &\defeq \sum_{\hat{\ell}}\alpha_{\ell,\hat{\ell}}\left.D_{2t}N_{\hat{\ell}}\right|^n_{\jv} + \sum_{m}\beta_{\ell,m}D_{0t}\Ev^n_{\jv}\cdot D_{0t} \Pv^n_{m,\jv}+ \sum_{m}\beta_{\ell,m}\Ev^n_{\jv}\cdot D_{+t}D_{-t} \Pv^n_{m,\jv}.\label{eqn:2-accurate-Ntt}
\end{align}
\end{subequations}
